# Supplementary material for: A Two-Stage Approach towards Generalization in Knowledge Base Question Answering
Source: arXiv:2111.05825 source file (2021-11-17)
Supplement: Supplementary file 1 [file appendix.tex]

\appendix

\section{Appendix}

Optionally include extra information (complete proofs, additional experiments and plots) in the appendix.
This section will often be part of the supplemental material.
